# Supplementary material for: Augmenting medical image classifiers with synthetic data from latent diffusion models
Source: arXiv:2308.12453 ancillary file (2023-08-23)
Supplement: Supplementary file 1 [file supplement.pdf]

# AUGMENTING MEDICAL IMAGE CLASSIFIERS WITH SYNTHETIC DATA FROM LATENT DIFFUSION MODELS

Supplement to: Sagers LW, Diao JA, and Melas-Kyriazi L, et al. "Augmenting medical image classifiers with synthetic data from latent diffusion models." This appendix has been provided by the authors to give readers additional information about the work

Table S-1: **A.** Data source, real image counts, and synthetic image counts for four experimental setups in this study. **B.** Synthetic generation method, use of standard augmentations (image transforms), and test set definition for the same four setups. *For the rare disease simulation, more real images were included in the test set of the disease of interest. This number varied based on the number of real images used in training.

**A**

| **Experiment** | Data Source | # Real per Condition | # Synthetic per Condition |
|---|---|---|---|
| Synthetic images in Fitzpatrick 17k | Fitzpatrick 17k | 1 \| 8 \| 16 \| 32 \| 64 \| 128 \| 228 | 0 \| 10 |
| Dose-response | Fitzpatrick 17k | 16 \| 32 \| 64 | 0 \| 10 \| 25 \| 50 \| 75 |
| Synthetic images in Stanford DDI | Stanford DDI | All 560 training images used | 0 \| 10 |
| Rare disease simulation | Fitzpatrick 17k | 200 x 8 conditions<br>25 \| 50 \| 100 x 1 condition | 0 (upsample)<br>7 \| 3 \| 1 for "rare" condition |

**B**

| **Experiment** | Generation Method | Standard Augmentations | Test Set |
|---|---|---|---|
| Synthetic images in Fitzpatrick 17k | Inpaint \| inpaint-outpaint \| text-to-image | True \| False | 360 (40 per condition) |
| Dose-response | text-to-image | True \| False | 360 (40 per condition) |
| Synthetic images in Stanford DDI | inpaint \| inpaint-outpaint | True \| False | 96 (32 per FST bin) |
| Rare disease simulation | Inpaint \| inpaint-outpaint \| text-to-image | True \| False | 360+ (40 per condition*) |

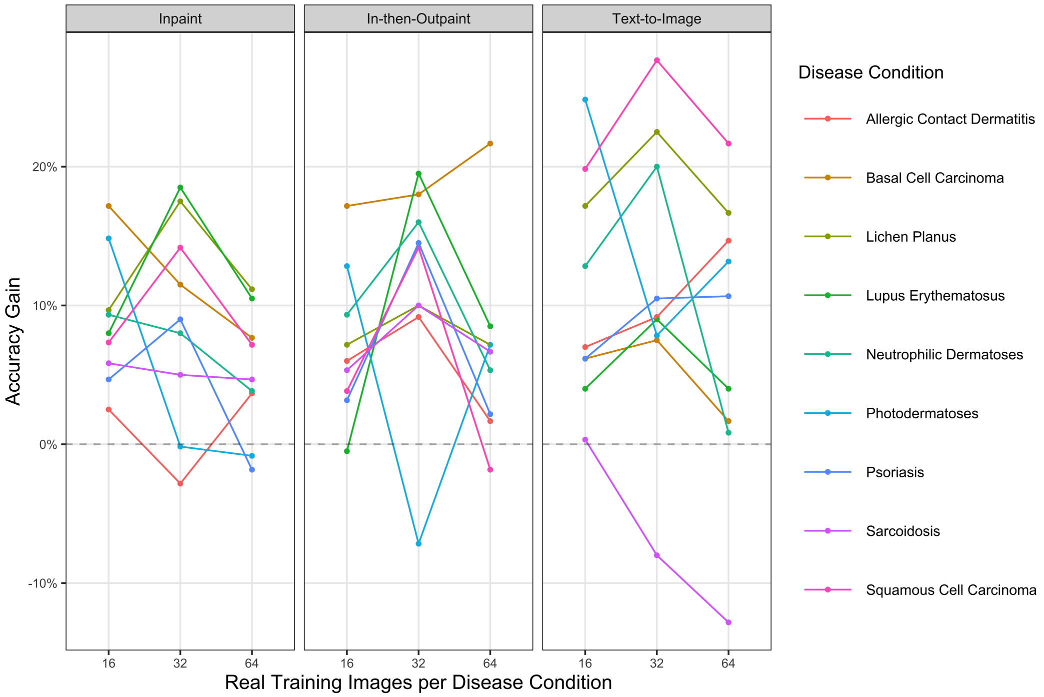


Figure S-1: Performance difference between models trained with and without synthetic augmentation for nine-way skin classification. Accuracy gain is defined as mean accuracy with synthetic augmentation minus mean accuracy without synthetic augmentation on a held-out test set. All models were trained using image transforms. Results are stratified by real image count (16, 32, or 64), disease condition, and generation method. Synthetic augmentation was performed using one of three methods: inpaint only, in-then-outpaint, and text-to-image. Model accuracy is averaged across five runs on a balanced, held-out test set of 360 images.

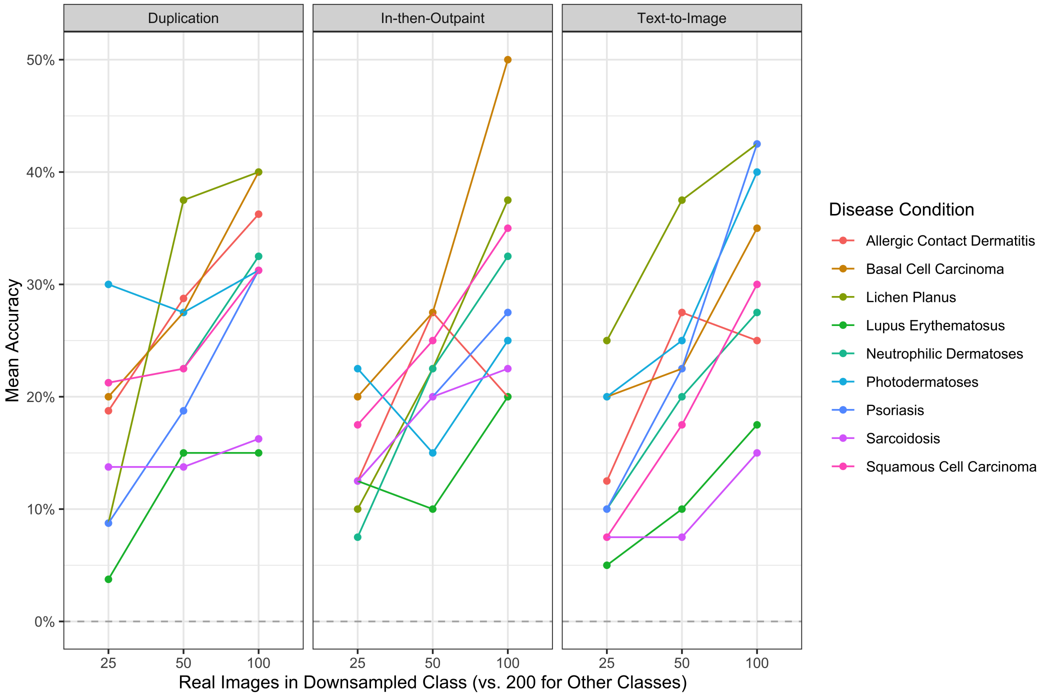


Figure S-2: Performance of models trained for nine-way skin classification with one class downsampled by 2, 4, or 8-fold. Results are stratified by disease condition and by upsampling strategy, including simple duplication and synthetic augmentation using in-then-outpainting or text-to-image. Model accuracy is averaged across five runs on a balanced, held-out test set of 360 images. Synthetic augmentation was performed using one of three methods: inpaint only, in-then-outpaint, and text-to-image.

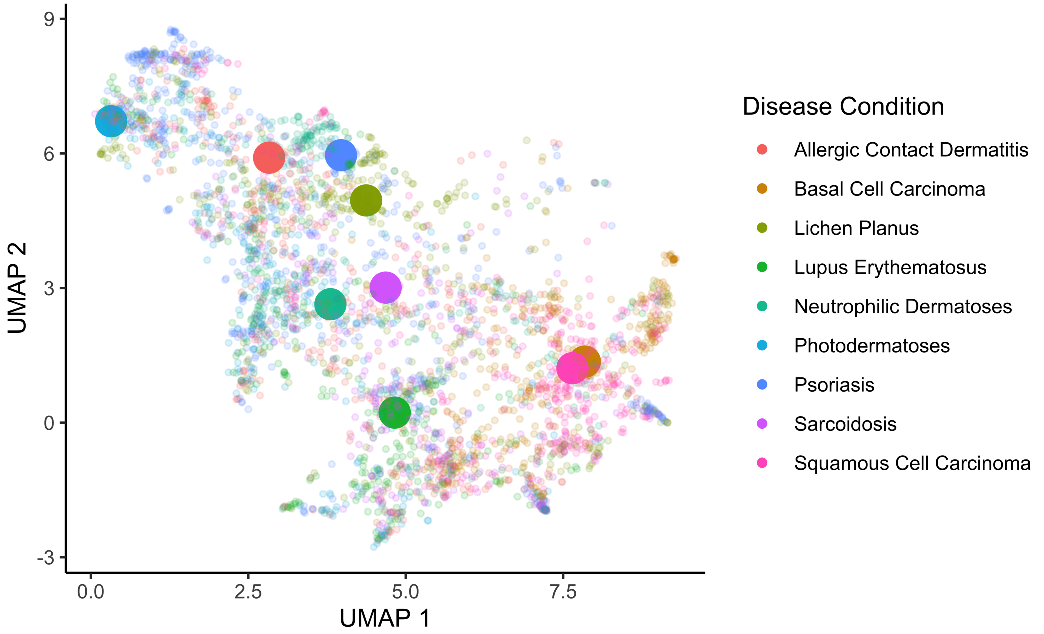


(A) Real images by disease condition

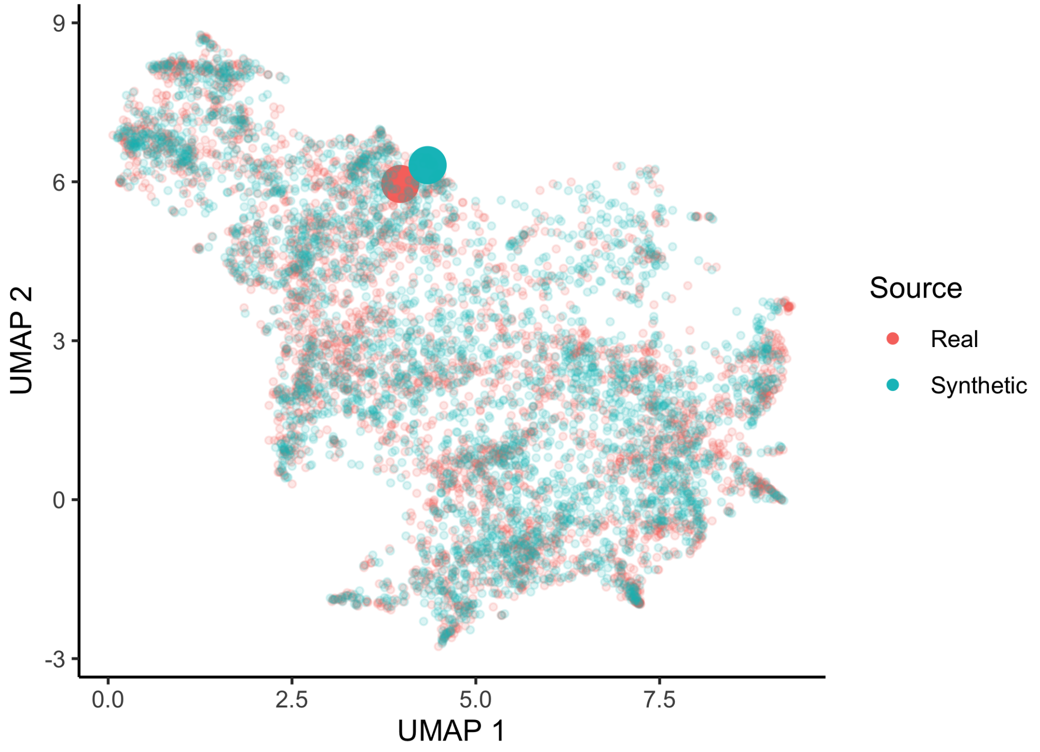


(B) Real versus synthetic images

Figure S-3: **A.** Dimensionality reduced representation of image embeddings for real and synthetic images produced using uniform manifold approximation and projection (UMAP) and colored by disease condition, with overlaid points corresponding to randomly selected examples in Figure 2A **B.** Same as A, but colored to indicate real or synthetic data, with an overlaid pair of points corresponding to the same examples in Figure 2B.

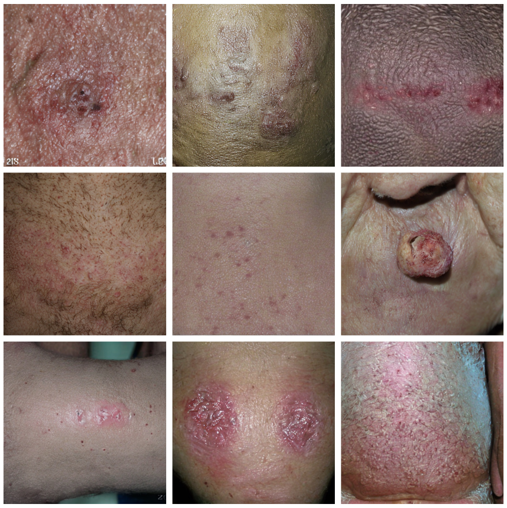

(A) Text-to-image generated images

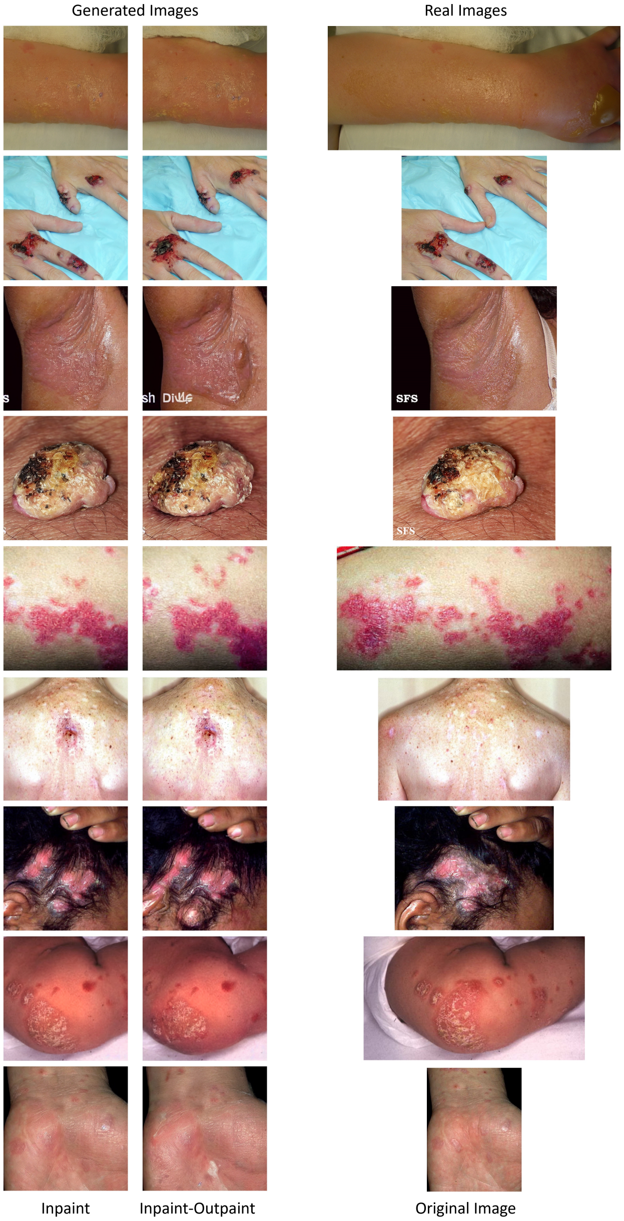


(B) Inpaint & inpaint-outpaint generated images vs real images

Figure S-4: **A.** Examples of synthetic images generated with the text-to-image method. The labels used for each image were, from left to right: **top row:** basal cell carcinoma, lupus erythematosus, sarcoidosis **middle row:** allergic contact dermatitis, photodermatoses, squamous cell carcinoma **bottom row:** lichen planus, neutrophilic dermatoses, psoriasis. **B.** Examples of synthetic images generated with the inpaint and inpaint-outpaint methods (left), compared with the original real reference images (right). From top to bottom, the conditions shown are: photodermatoses, neutrophilic dermatoses, allergic contact dermatitis, squamous cell carcinoma, sarcoidosis, basal cell carcinoma, lupus erythematosus, psoriasis, lichen planus.
